# Supplementary material for: Leveraging LLMs for Synthesizing Training Data Across Many Languages in Multilingual Dense Retrieval
Source: arXiv:2311.05800 source file (2024-04-15)
Supplement: Supplementary file 1 [file annotation-guidelines.pdf]

# Annotation Guidelines for SWIM-IR

Nandan Thakur

June 2nd 2023

- The goal of this task is to evaluate the quality of LLM-generated (PaLM 2-S) generated questions.
- Every annotator will receive a set of annotations containing the wikipedia paragraph and the question in the  $\text{\$}\{target\_language\}$ .
- Annotators should read each annotation carefully and provide feedback on the following:
  - The **fluency** of the question.
  - The **adequacy** of the question.
  - The **language** of the question.
- Annotators should be respectful and professional in their feedback.
- Annotators should complete all annotations within the allotted duration.

Here below we define the following terms:

## Fluency

| Rating Level | Explanation                                                                                                        |
|--------------|--------------------------------------------------------------------------------------------------------------------|
| 2 (Flawless) | Perfect use of $\text{\$}\{target\_language\}$ with no mistakes at all.                                            |
| 1 (Good)     | Few or minor spelling or grammar mistakes; the text is still mostly understandable and readable.                   |
| 0 (Poor)     | Many or serious spelling, grammar, or other mistakes, which make the text difficult to understand or hard to read. |

## Adequacy

| Rating Level | Explanation                                                                              |
|--------------|------------------------------------------------------------------------------------------|
| 2 (Relevant) | Highly related to the wiki passage. The question can be answered using the wiki passage. |

|                         |                                                                                                            |
|-------------------------|------------------------------------------------------------------------------------------------------------|
| <b>1</b> (Moderate)     | The question is somewhat related to the wiki paragraph, the question cannot be answered using the passage. |
| <b>0</b> (Not Relevant) | The question is not at all related to the wiki passage.                                                    |

### **Language**

| <b>Rating Level</b> | <b>Explanation</b>                                                              |
|---------------------|---------------------------------------------------------------------------------|
| <b>2</b> (Flawless) | The whole question is perfectly in the $\${target\_language}$ .                 |
| <b>1</b> (Good)     | Code-switching occurs with part of the question in the $\${target\_language}$ . |
| <b>0</b> (Poor)     | The whole question is not at all in $\${target\_language}$ .                    |

Thank you for your participation in this task!
